# Supplementary material for: Optical probing of magnons and phonons in Ni80Fe20 nanodot arrays
Source: arXiv:2601.10892 source file (2026-01-15)
Supplement: Supplementary file 1 [file SM.pdf]

# Supplementary Information
# Optical probing of magnons and phonons in $Ni_{80}Fe_{20}$ nanodot arrays

A. Adhikari,[1] P. Graczyk*,[2] A. K. Chaurasiya,[1,3] S. Mondal,[1] J. W. Kłos,[4] and A. Barman*,[1,5]

[1)] *Department of Condensed Matter and Materials Physics, S. N. Bose National Centre for Basic Sciences, Block JD, Sector III, Salt Lake, Kolkata 700106, India*

[2)] *Institute of Molecular Physics, Polish Academy of Sciences, M. Smoluchowskiego 17, 60-179, Poznan, Poland*

[3)] *Department of Physics, University of Gothenburg Box 100, 405 30 Gothenburg, Sweden*

[4)] *ISQI, Faculty of Physics and Astronomy, Adam Mickiewicz University Poznan, Uniwersytetu Poznańskiego 2, 61-614, Poznań, Poland*

[5)] *Department of Physics, School of Natural Sciences, Shiv Nadar Institution of Eminence (Delhi NCR), Dadri UP 201314, India*

(*Electronic mail: graczyk@ifmpan.poznan.pl, abarman@bose.res.in, anjan.barman@snu.edu.in)

**SI-I: Time-resolved MOKE spectra showing the reflectivity and Kerr rotation together with the SEM images of the three different samples S1, S2, and S3.**

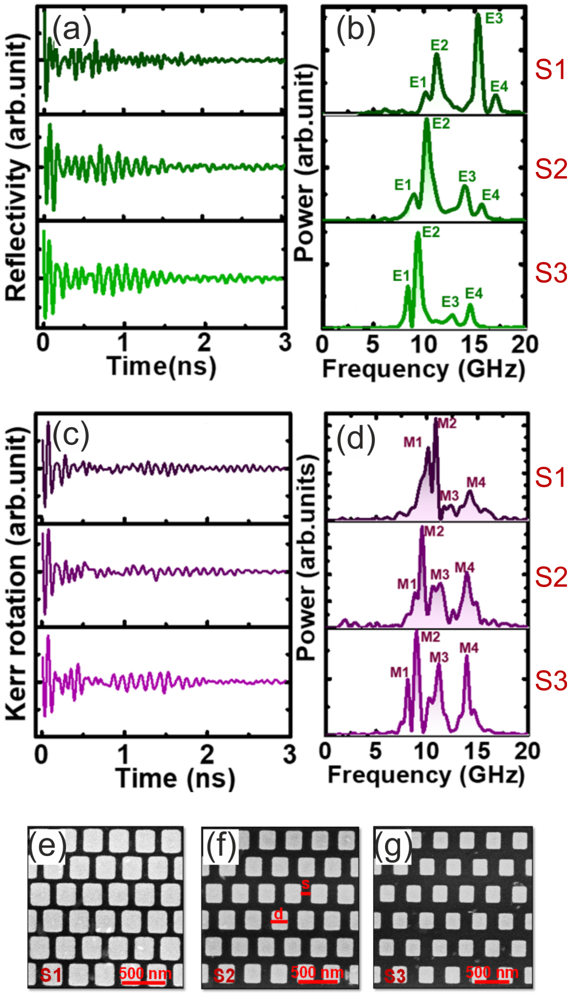


Supplementary Figure 1. Background subtracted time-resolved (a) reflectivity and (c) Kerr rotation changes indicating acoustic (SAW) and magnetization (SW) dynamics respectively detected for three different samples S1, S2, and S3 at a magnetic field of $H_{ext}$ = 1.75 kOe. (b) and (d) are fast Fourier transformed (FFT) power spectra of the time-resolved reflectivity and Kerr rotation, respectively. The peaks indicate the frequencies of the excited SW and SAW modes. (e-g) Scanning electron micrographs of $Ni_{80}Fe_{20}$(Py) nanodots arranged in hexagonal geometry (samples S1, S2, S3) with lattice constants $d+s$: 300 nm (e), 350 nm (f), 400 nm (g).

**SI-II: The variation of SAW frequency as a function of lattice constant.**

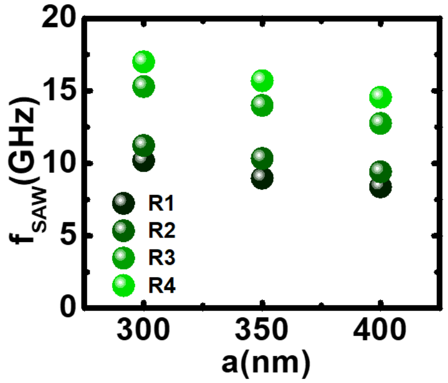


Supplementary Figure 2. Experimentally estimated SAW frequencies as a function of lattice constants.

**SI-III: Time-resolved MOKE showing the Kerr rotation for a continuous Py layer at different magnetic fields.**

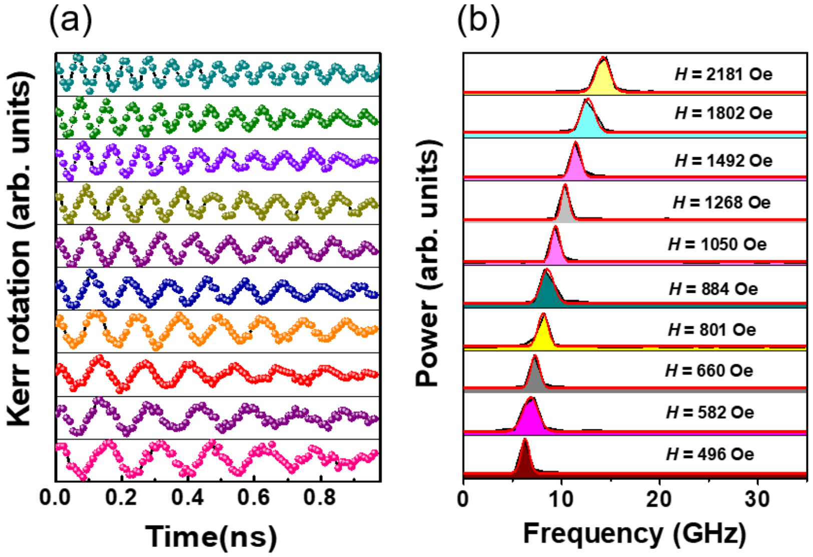


Supplementary Figure 3. Time-resolved Kerr rotation data (a) along with their FFT power spectra (b) for a 20-nm-thick continuous Py film at varying bias magnetic field. A single uniform precessional mode is observed for all bias field values.

## SI-IV: Magnetic field dependence of the time-resolved Kerr rotation change for sample S3

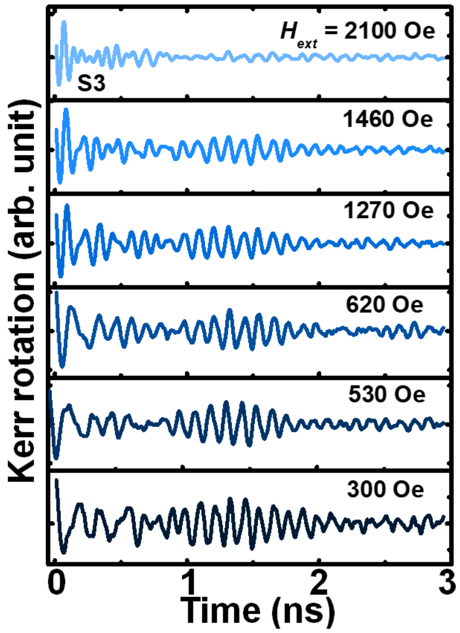


Supplementary Figure 4. Background subtracted time-resolved Kerr rotation change showing the presence of non-decaying magnetization SW dynamics for S3 with decreasing magnetic field of $H_{\rm ext}$ .

## SI-V: The coupled surface phonon - magnon dispersion relation for the cubic geometry

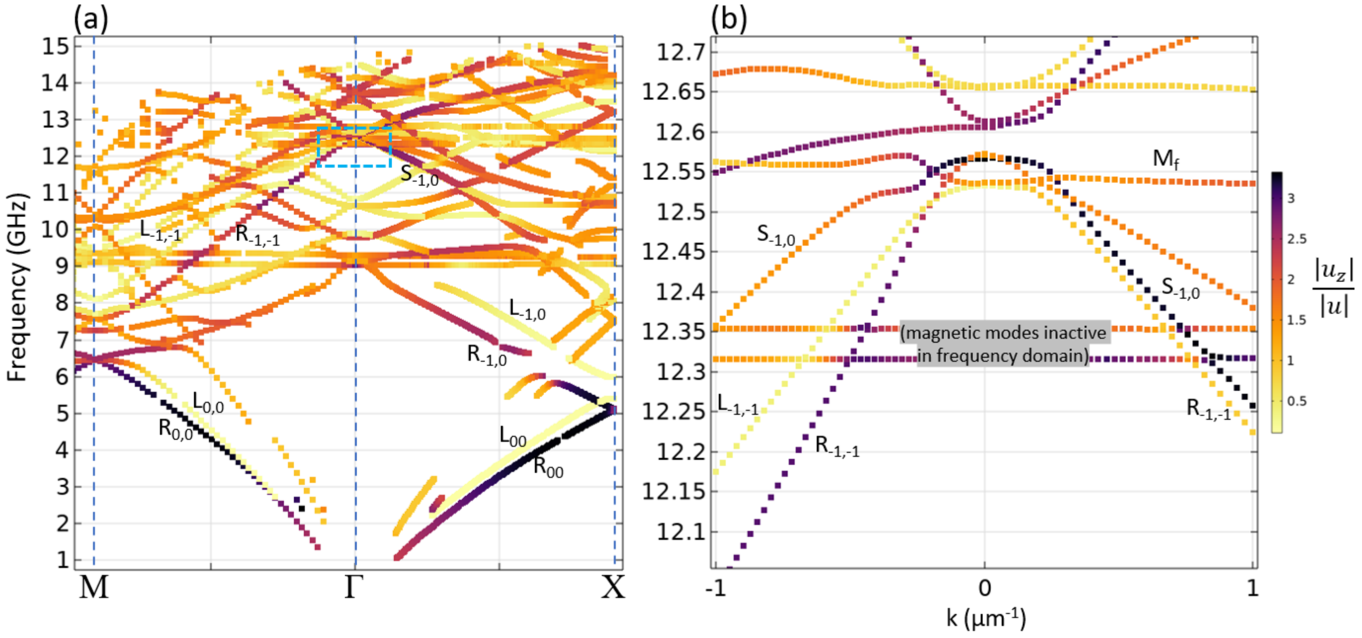


Supplementary Figure 5. (a) The magnetoelastic dispersion relation presenting the coupling between the SAWs and SWs modes at 143 mT in square lattice of Py dots. The Rayleigh (R), Love (L) and Sezawa (S) modes are labelled using the $x-$ and $y-$indices of the reciprocal lattice vectors in square lattice when folding into the first Brillouin zone; (b) the zoomed part of the dispersion relation around $\Gamma$ point, indicated by the blue dashed rectangle in (a). The color of points indicate amplitude of the out-of-plane displacement.
